# Supplementary material for: Nondeterministic Behaviours in Double Categorical Systems Theory
Source: arXiv:2502.02517 source file (2026-01-11)
Supplement: Supplementary file 1 [file appendix_connections.tex]

\section{Connections with classical settings}\label{appendix_connections}

In this section, we discuss connections between our double categorical framework and the notions described in section \ref{section_classical}
\subsection{The coalgebraic point of view}

\subsection{Symmetric monoidal categories as simple systems theories}
